# Supplementary material for: LaHAR: Latent Human Activity Recognition using LDA
Source: arXiv:2011.11151 source file (2020-11-23)
Supplement: Supplementary file 1 [file appendix.tex]

The classification results in terms of precision and recall obtained by Anguita et al~\cite{anguita2013public}. are presented in table \ref{bas1}. Similar to our results, the authors obtain 100\% recall for the LAYING class. Also their results present some misclassifications between the class SITTING and STANDING, what the authors attributed to the position of the sensor while the user was performing the activity. Futhermore, LDA produced similar results on the three dynamic activities WALKING, WALKING\_UPSTAIRS and WALKING\_DOWNSTAIRS. However, the degree of misclassification between the activities SITTING and STANDING was higher for LDA.
\begin{center}
\begin{table*}[h]
\leftskip=0.1cm
\begin{tabular}{|c|cccccc|c|}
\hline
\backslashbox{Actual}{Predicted} &  WA & WU & WD & SI &  ST & LA &Recall\\
\hline
WA &492 &     1 &     3 & 0 &     0 & 0&99\% \\
WU & 18 & 451 & 2 & 0 &     0 & 0& 96\%\\
WD &4 &6 &410 &0 &     0 &  0& 98\%\\
SI &  0 &  2 &  0 &    423 &  57 &     0& 88\%\\
ST &     0 &     0 &  0 &     14 &  518 &     0& 97\%\\
LA &     0 &  0 &     0 &     0 &    0 &     537& 100\%\\\hline
Precision &96\%&98\%&99\%&97\%&90\%&100\%&96\%\\
\hline
\end{tabular}
\caption{Confusion matrix of the classification results on the test data using SVM \cite{anguita2013public}}
\label{bas1}
\end{table*}
\end{center}
Another baseline we used to benchmark our result is the codebook method. The codebook is a state-of-the-art method for extracting features to characterize sequences for the sake of HAR \cite{shirahama2017}. The codebook method consists of three main steps: Subsequence extraction: First, numerous subsequences are collected from sequences through the sliding window technique. b) Clustering: Abundant subsequences are grouped into clusters to increase the variance among them. The cluster centers, called, codewords represent specific local patterns of the subsequences in that cluster. c) Histogram construction: Finally, sequences are represented with histogram-type feature vectors expressing the distribution of codewords in the sequences. The histogram-type feature vectors are used as inputs to fit a classification model. The histogram-type features extracted using the codebook method was fitted to SVM and RFC (Random Forest Classifier). Another experiment we did consisted to provide the vector of posterior distributions of activity instances as feature to classification model. The two classification models SVM were trained and compared with the results of the codebook method as well with the results obtained from using LDA alone. \ref{tab:allme} shows the results of all experiments that we conducted.

\begin{center}
\begin{table}[H]
\leftskip=2cm
\begin{tabular}{|l|l|}
\hline
 \textbf{Methods}&\textbf{Accuracy}\\ \hline
 {Anguita et al.}& \textbf{96}\%\\ \hline
 {Codebook+SVM } &89\%\\ \hline
 {LDA+SVM}& 92\%\\ \hline
 {Codebook+RFC}&89\% \\ \hline
 {LDA+RFC}&90\% \\ \hline
 {LDA}&91\% \\ \hline
 
\end{tabular}
\caption{LDA with SVM and RFC}
\label{tab:allme}
\end{table}
\end{center}
Table \ref{tab:allme} shows that the LDA model, although unsupervised can predict the class of activity instances with an accuracy of recognition comparable to supervised algorithms. Also, the features created with LDA are more meaningful for classification compared to those extracted using the codebook

\subsection{Discussion}
It is imperative to examine if the LDA's conception of documents as mixtures of topics also applies to sequences. Figure~\ref{dist:activ} shows plots of the activity class distributions for one instance of
each activity class. From these plots, one can observe that the activity class WALKING also encompasses some components of activities WALKING\_DOWNSTAIRS and WALKING\_UPSTAIRS as these three activities are very similar. On the other hand, the distribution of the activity SITTING is focused on one activity. 
 \begin{figure*}
\centering
  \begin{subfigure}{0.4\textwidth}
    \includegraphics[width=\textwidth]{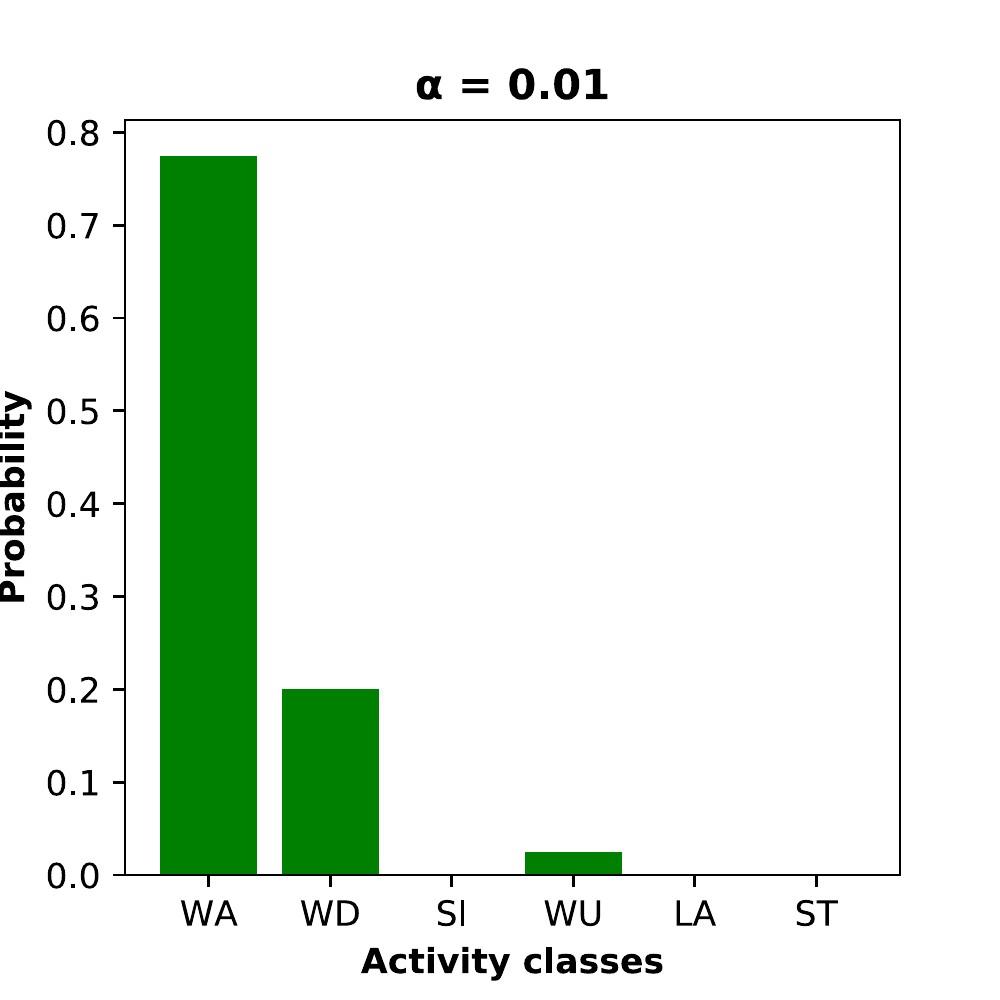}
    \caption{Instance of activity WALKING}
    \label{fig:wu2c1}
  \end{subfigure}
  \begin{subfigure}{0.4\textwidth}
    \includegraphics[width=\textwidth]{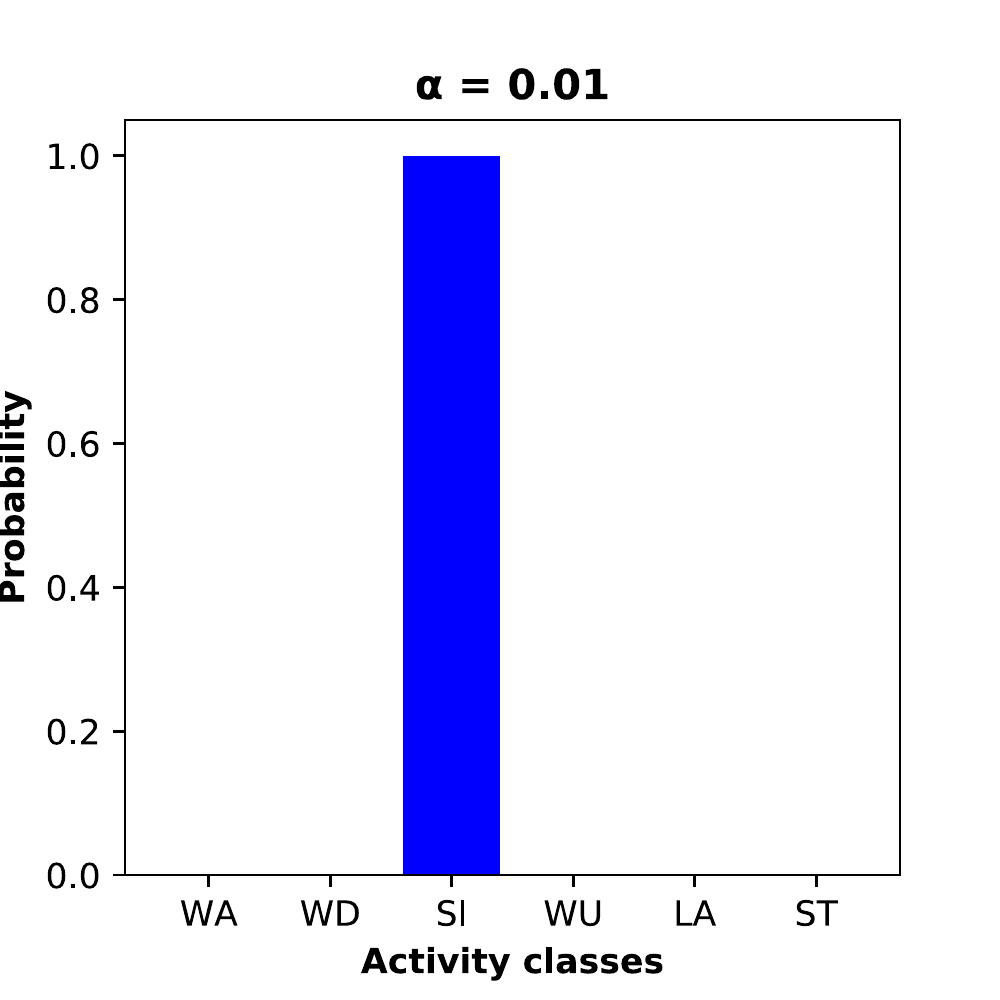}
    \caption{Instance of activity SITTING.}
    \label{fig:si2c1}
  \end{subfigure}
  \caption{Activity distribution for single data sequences}
  \label{dist:activ}
  \end{figure*}

Figure \ref{fig:swd2c} illustrates the distribution of the 20 most frequent \textit{SWs} in the activity datase. It can be observed that there are only few \textit{SWs} that are very frequent across all activities, and the vast majority of \textit{SWs} are less frequent. This aligns with the way words are distributed in in textual documents.

\begin{center}
\begin{figure}[H]
  \includegraphics[width=0.5\textwidth]{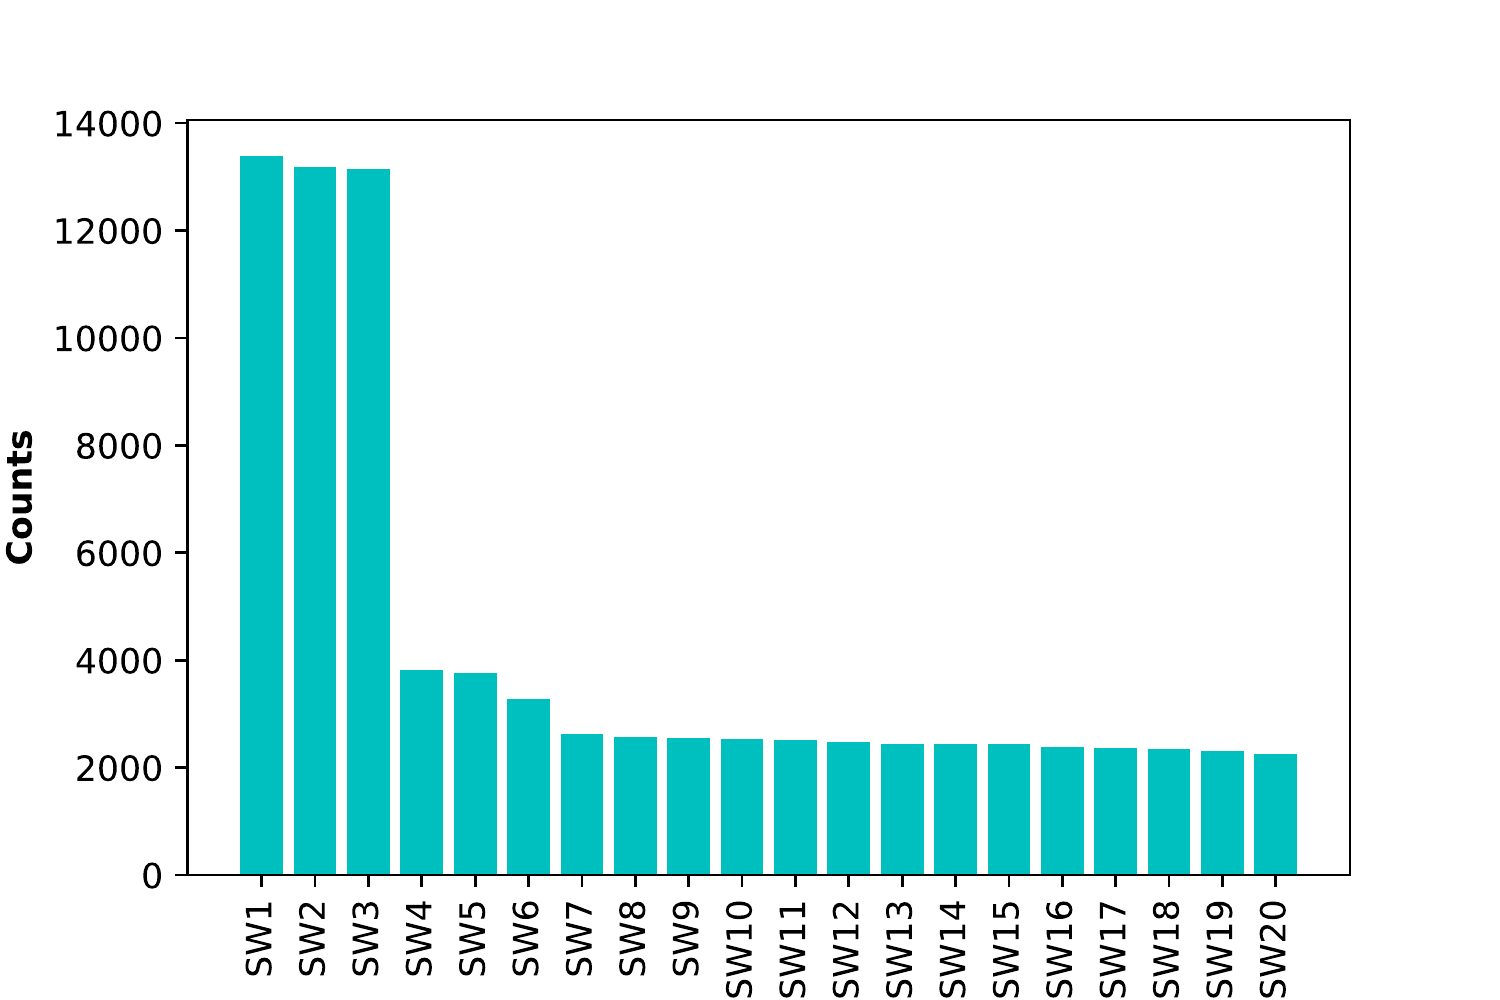}
  %\vspace{-0.1in}
  \caption{Distribution of the 20 most frequent \textit{SWs}}
  \label{fig:swd2c}
\end{figure}
\end{center}
